# Supplementary material for: LPMM: Intuitive Pose Control for Neural Talking-Head Model via Landmark-Parameter Morphable Model
Source: arXiv:2305.10456 source file (2023-05-17)
Supplement: Supplementary file 1 [file 6_appendix.tex]

In the supplementary material, we provide additional details surrounding our pipeline, along with practical issues surrounding the implementation of our work. We also provide additional insights we gained throughout this research. We strongly recommend watching the supplementary video, for more head pose editing results.

\section{LPMM implementation details}

\begin{figure*}[t!]
    \centering
    \vspace{-0.4cm}
    \includegraphics[width=1\linewidth]{supp/pca_components_5.jpg}
    \vspace{-0.6cm}
   \caption{Each row represents the linear interpolation results for different LPMM parameters ($p_1$ ~ $p_5$). $p_1$, $p_2$, and $p_5$ are each responsible for controlling yaw, roll, and pitch orientation. $p_3$ and $p_4$ are also related to head orientation, but contains unwanted shape information e.g. jaw width.}
    \vspace{-0.2cm}
   \label{fig:PCA_components}
\end{figure*}

% 각 row는 LPMM의 parameter를 순서대로 interpolation 시킨 결과이다. 1번,2번,5번 parameter는 각각 head orientation인 yaw, roll, pitch가 control 되는것을 확인 할 수 있다. 3번,4번 parameter는 턱 넓이와 같은 shape과 관련된 정보가 embedding 되어 있음을 알 수 있다.

\begin{figure*}[t!]
    \centering
    \vspace{-0.4cm}
    \includegraphics[width=1\linewidth]{supp/param34_interpolation.jpg}
    \vspace{-0.6cm}
   \caption{We tested the head pose editing results for different values of $p_3$ and $p_4$, with images generating using LPD~\cite{burkov2020@lpd} as our backbone generator. It can be observed that thanks to the identity-pose disentanglement power of talking head generators, the identity of the generated faces are not distorted despite $p_3$ and $p_4$ contains shape information.}
    \vspace{-0.2cm}
   \label{fig:param34}
\end{figure*}

% shape이 조절되는 3번째 parameter와 4번째 parameter를 interpolation 시킨 결과 identity distortion이 발생되지 않는다. 이는 우리의 method가 talking head generator의 identity- disentangle power를 활용 할 수 있기 때문이다.

Prior to training, we defined the landmark-parameter morphable model (LPMM) based on the extracted PCA components from the Voxceleb datasets ~\cite{Nagrani17@vox1, chung2018voxceleb2}. We assumed that it is possible to extract parameters that are only responsible for the head orientation movements, by basing on video-based datasets. 

According to EG3D~\cite{chan2022@eg3d}, the FFHQ dataset contains a strong correlation between orientation and facial expressions, as individuals facing the camera directly have a tendency to smile more than those who are not facing the camera. However, VoxCeleb datasets consist of videos containing multiple frames of the same identity with differing orientations and facial expressions, so we assumed that by using VoxCeleb, it is possible to eliminate such biases. The extracted PCA components indeed displayed a clear division between head orientation and facial expressions. As shown in Figure~\ref{fig:supp_teaser} and Figure~\ref{fig:PCA_components}, the 1st, 2nd, and 5th parameters are each responsible for yaw, roll, and pitch orientations, without controlling facial expressions.

\section{Training details}

As noted in the main paper, we deploy a two-stage training scheme for our model. In the first stage, LP-regressor was optimized using Adam with a learning rate of 1e-4. The training was carried out on a single RTX 2080 GPU, and took 40 epochs for convergence.

In the second stage, LP-adaptor was optimized with the same optimizer setting as LP-regressor. Modeled as a three-layer perceptron, the output dimension for each linear layer is twice the input dimension, and the final output dimension is fixed to the chosen talking head generator’s pose vector dimension. We use $\lambda_{rgb}=1$, $\lambda_{pose-reg}=1$ for hyperparameters. Convergence occurs within a single epoch. Since the LP-adaptor’s training includes calculating the gradients for the talking head generator, training hours are dependent on the generator choices; using a single RTX 2080 GPU, it took about 3 days for the LPD~\cite{burkov2020@lpd} model and 9 days for LIA~\cite{wang2021@lia} model.

In practice, few-shot learning of the talking-head generator model for an unseen identity might be required. When using LPD~\cite{burkov2020@lpd} as the generator, usually 5$\sim$10 facial images are needed for training, which takes about 15$\sim$20 minutes on a single RTX 2080 GPU. LIA~\cite{wang2021@lia} doesn't requires any training, and can be used for any facial image. 

For comparison we implemented StyleRig ourselves, due to no publicly available StyleRig implementations. As StyleRig needs synthetic data from StyleGAN ~\cite{karras2019stylegan}, we generated 200k training samples from randomly sampled latent vectors. Given these $(w, I_w)$ pairs, we train StyleRig according to the paper ~\cite{tewari2020@stylerig}. Further comparison results between our method and StyleRig can be shown in Figure \ref{fig:stylerig1},\ref{fig:stylerig2}.

\section{Ablation Study}

In this section, we evaluate the contribution of different losses used during the training of our method. Since the training of the LP-regressor is rather straightforward, and we followed the official training pipelines for each talking head generator, we focus on the LP-adaptor training.

We evaluated the Normalized Mean Error (NME) results for different loss settings. Specifically, we wanted to measure the effectiveness of pose regularization loss ($\mathcal{L}_{\text{pose-reg}}$), and if using $\ell_1$-loss in the RGB space ($\mathcal{L}_{\text{RGB}}$) produces a meaningful difference from the latent space ($\mathcal{L}_{\text{latent}}$). The results can be seen in Table~\ref{tab:LPA_losscomp}. As displayed, the addition of pose regularization loss provides a meaningful level of decreased NME when $\mathcal{L}_{\text{RGB}}$ is used. We concluded that using both $\mathcal{L}_{\text{RGB}}$ and $\mathcal{L}_{\text{pose-reg}}$ provides the best quality and head pose editability, and used it as our default setting.

% Please add the following required packages to your document preamble:
% \usepackage{graphicx}
\begin{table}[]
\resizebox{\columnwidth}{!}{%
\begin{tabular}{l|cccc}
\hline
 &
  \multicolumn{1}{l}{$\mathcal{L}_{\text{latent}}$} &
  \multicolumn{1}{l}{$\mathcal{L}_{\text{latent}}, \mathcal{L}_{\text{pose-reg}}$} &
  \multicolumn{1}{l}{$\mathcal{L}_{\text{RGB}}$} &
  \multicolumn{1}{l}{\textbf{$\mathcal{L}_{\text{RGB}}, \mathcal{L}_{\text{pose-reg}}$}} \\ \hline
\textbf{LPD ~\cite{burkov2020@lpd}} &
  3.66 &
  3.73 &
  3.64 &
  \textbf{3.60} \\ \hline
\textbf{LIA ~\cite{wang2021@lia}} &
  4.75 &
  4.60 &
  4.64 &
  \textbf{4.54}
\end{tabular}%
}
\caption{NME comparison between different loss functions used for LP-Adaptor training. }
\label{tab:LPA_losscomp}
\end{table}

% \begin{table}[]{
%     \resizebox{\textwidth}{!}{%
%         \begin{tabular}{l|cc}
%         \hline & \multicolumn{1}{l}{\textbf{LPD ~\cite{burkov2020@lpd}}} & \multicolumn{1}{l}{\textbf{LIA ~\cite{wang2021@lia}}} \\ 
%         \hline $\mathcal{L}_{\text{latent}}$  & 3.66 & 4.75  \\ \hline
%         $\mathcal{L}_{\text{latent}}, \mathcal{L}_{\text{pose-reg}}$ & 3.73                             & 4.60                             \\ \hline
%         $\mathcal{L}_{\text{rgb}}$                                   & 3.64                             & 4.64                             \\ \hline
%         \textbf{$\mathcal{L}_{\text{rgb}}, \mathcal{L}_{\text{pose-reg}}$} & \textbf{3.60} & \textbf{4.54} \\ \hline
%         \end{tabular}%
%     }
% }
% \caption{NME comparison between different loss functions used for LP-Adaptor training. }
% \label{tab:LPA_losscomp}
% \end{table}

\section{Discussion}

As displayed in Figure~\ref{fig:PCA_components}, for certain LPMM parameters, shape information (that is not relevant to head pose) is also edited during parameter interpolation. We attribute this issue to the fact that facial landmarks can sometimes contain identity-specific information e.g. jaw width, which is also processed and extracted during the creation of LPMM. However, this tendency rarely impacts the performance of our pipeline, as we use neural talking head models that directly address the identity-pose disentanglement problem ~\cite{burkov2020@lpd, wang2021@lia}. For instance, LIA ~\cite{wang2021@lia} encodes head pose motion separately from any identity information, by constructing motion in the form of the linear combination of latent codes. Using such talking head models as image generators and pose encoders prevent the distortion of human identity during our method, minimizing the risk of unwanted changes. Additional results can be seen in Figure ~\ref{fig:param34}.

\begin{figure*}[t!]
    \centering
    \vspace{-0.4cm}
    \includegraphics[width=0.95\linewidth]{supp/stylerig_big1.jpg}
    \vspace{-0.2cm}
   \caption{Comparison to StyleRig  ~\cite{tewari2020@stylerig}. The first row shows 3DMM visualization. The StyleRig results were created from our StyleRig implementations, and ours results were created using LIA ~\cite{wang2021@lia} generator as a backbone. Our approach is on par with StyleRig for head orientation(yaw, pitch), produces a better pose transfer for in-place rotations(roll) and is identity-consistent.}
    \vspace{-0.2cm}
   \label{fig:stylerig1}
\end{figure*}
\begin{figure*}[t!]
    \centering
    \vspace{-0.4cm}
    \includegraphics[width=0.95\linewidth]{supp/stylerig_big2.jpg}
    \vspace{-0.2cm}
   \caption{Comparison to StyleRig  ~\cite{tewari2020@stylerig}. The first row shows 3DMM visualization. The StyleRig results were created from our StyleRig implementations, and ours results were created using LIA ~\cite{wang2021@lia} generator as a backbone. Our approach is on par with StyleRig for head orientation(yaw, pitch), produces a better pose transfer for in-place rotations(roll) and is identity-consistent.}
    \vspace{-0.2cm}
   \label{fig:stylerig2}
\end{figure*}
